# Supplementary material for: Improving the Design of Linear Controllers for Homogeneous Platooning under Disturbances
Source: arXiv:2312.14897 source file (2023-12-22)
Supplement: Supplementary file 1 [file 9_appendix.tex]

\appendices

% Appendixes, if needed, appear before the acknowledgment.
